# Supplementary material for: Efficient LSM-Tree Key-Value Data Management on Hybrid SSD/HDD Zoned Storage
Source: arXiv:2205.11753 source file (2022-05-24)
Supplement: Supplementary file 1 [file appendix.tex]

\clearpage
\newpage

\appendix

\section*{Appendix}
\label{sec:appendix}

We report additional evaluation findings. 

\paragraph{Exp\#S1 (Impact of the migration rate).} Recall that in
\S\ref{subsec:migration}, we rate-limit the migration to reduce interference
with foreground traffic and ensure predictable latencies.  We now study the
impact of the migration rates on the tail latencies. We do not consider
application-hinted caching and use P+M as in Exp\#3. We vary the migration
rates from 1\,MiB/s to 64\,MiB/s. We load 200\,GiB of 1-KiB KV objects, and
run a workload with 50\% reads, 50\% writes, and $\alpha=0.9$.  We focus on 
the read latencies. 

Figure~\ref{fig:exp6_migthpt} shows the 99th, 99.9th, and 99.99th percentile
read latencies versus the migration rate. We show that the 99th percentile
latencies are comparable for all migration rates, with less than 10\% of
variations. The 99.9th percentile latency is the lowest for migration rates of
{\color{red}2\,MiB/s} and 4\,MiB/s, while the highest 99.9th percentile latency
is on the migration rate of 64\,MiB/s, which is {\color{red}23.0\% and 25.4\%
higher than those of 2\,MiB/s and 4\,MiB/s, respectively}. It shows that a
large migration rate increases the interference with foreground reads. The
99.99th percentile latencies show an increasing trend with the increasing
migration rate. The 99.99th percentile latency for 64\,MiB/s is
{\color{red}$2.04\times$} that of 1\,MiB/s.  Our default setting selects
4\,MiB/s as the migration rate for our evaluation without significantly
increasing the tail latency. 

\begin{figure}[!t]
\centering
\includegraphics[width=2in]{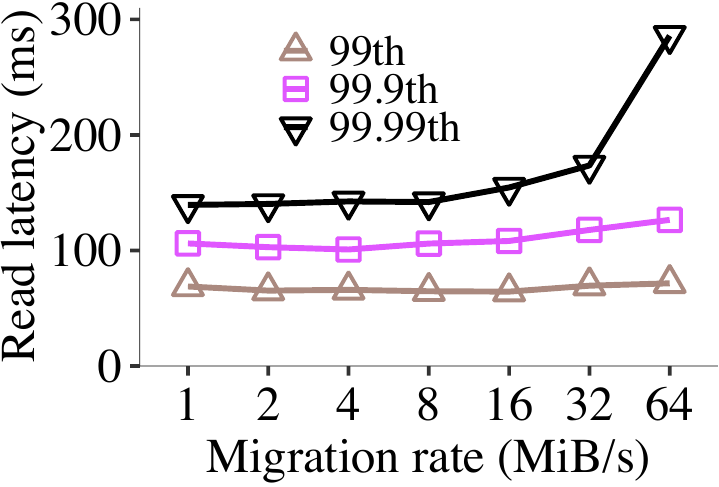}
\vspace{-3pt}
\caption{Exp\#S1 (Impact of the migration rate).}
\label{fig:exp6_migthpt}
\end{figure}

\begin{figure}[!t]
\centering
\includegraphics[width=2in]{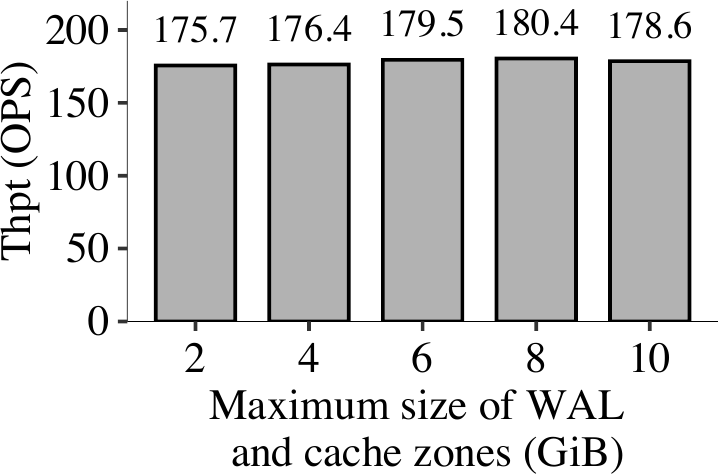} 
\vspace{-3pt}
\caption{Exp\#S2 (Impact of the maximum size of WAL and cache zones). }
\label{fig:exp7_cachesize}
\end{figure}

\paragraph{Exp\#S2 (Impact of the maximum size of WAL and cache zones).} Recall
that in \S\ref{subsec:caching}, \sysname reuses the SSD zones reserved for the
WAL for caching. We now study the impact of the maximum {\color{red} number} of
WAL and cache zones (denoted by $S$) by fixing the total SSD space as
{\color{red}21.0\,GiB, i.e., 20 SSD zones,} and varying $S$ from {\color{red}2
to 10}.  We run the workloads with 5\,M operations, with 50\% reads, 50\%
writes, and $\alpha=0.9$.  We examine the throughput of the last 1\,M
operations to ensure that the SSD cache is warmed up in these operations.
Figure~\ref{fig:exp7_cachesize} shows the results.  The performance does not
significantly change across different values of $S$. 
%different cache sizes. The reason is that although more cache zones save more
%frequently read SST blocks, the number of zones for saving SSTs shrinks
%accordingly.  Note that although not shown, too large SSD caches take long to
%fill all the cache zones; and it wastes SSD zones if the workload becomes
%write-intensive and performs few KV lookups. Therefore, we argue that reusing
%the zones reserved for WAL is enough for the SSD cache. 
